# Supplementary material for: VRDSynth: Synthesizing Programs for Multilingual Visually Rich Document Information Extraction
Source: arXiv:2407.06826 source file (2024-07-09)
Supplement: Supplementary file 1 [file suplementary_material.tex]

%\subsection{Information Extraction from Visually Rich Documents}
%\label{subsec:bg_ie}
%\marc{what is key, value}
%\bachle{Give example. Also, define semantic and spatial relation. Don't expect readers to be familiar with those terms.}
In this section, we formally define the information extraction (IE) problem from virtually rich documents (VRDs) following~\cite{Madashi2019, Jaume2019} and subsequently provide the background on constituent parts of \toolname that we use. In particular, we will describe Graph Neural Networks (GNNs)~\cite{} that learn to represent VRDs as graphs, GNN Explainer~\cite{} that explains the models learned from GNNs, and a DSL and program synthesizer~\cite{} used to synthesize programs that rectify errors of the GNN's model.

\begin{definition}
Information Extraction. Visually rich documents (VRDs) can be represented as text segments, each of which contains text content and the bounding box of the segment. Let a VRD be defined as a set of $N$ text segments $\langle t_i \rangle$. Each segment $t_i$ is represented as a tuple of $(x, y, w, h, text)$ which denotes coordinates of the segment in the VRD, the width, height and content of the segment respectively. Given $f$ denoting the desired field to extract from a VRD, information extraction outputs a set of text segments $\langle t_f \rangle$ which are associated with the desired field $f$.
\end{definition}

In this work, we represent each VRD as a graph, wherein each node represents a text segment and an edge between two nodes represents the spatial relation among the nodes, e.g., the relative position (alignment) between the nodes' text segments on the VRD. Nodes that share some common property can be categorized into groups. The IE problem is now equivalent to the problem of querying graphs to retrieve relevant group of nodes associated with a desired property $f$. To achieve this, we use a Graph Neural Network (GNN) to learn a model for node classification. We next explain the GNN that we use~\cite{Such2017} which enables to incorporate both semantic and spatial relations among nodes.

\textbf{Graph Neural Networks (GNNs)}. GNNs~\cite{Such2017, Zhang} are a class of neural network adapted for graph structures. In this work, we adapt the Chebyshev-approximation of Graph Convolution Network (GCN) as proposed in \cite{Zhang2016} and its variant to accommodate multiple types of edges as proposed in \cite{Such2017}. In order to employ GCN for documents IE, the document need to be transformed into a graph. The most common way for building graph from the document is to represent each segment as a node, the other information such as textual information, visual information are encoded as feature vector of the node. After the graph representation of document is generated, GCN is employed to incorporate graph's information, then the IE is formulated as graph node classification. 

\marc{How GNN is employed?}

%\subsection{GNN Explainer}
\textbf{GNN Explainer}. GNN explainer \cite{Cranmer2020} is a model-agnostic approach to provide explanation for GNN-based models. Explanation is provided under the form of adjacency and feature mask through an optimization process. GNN Explainer takes input as adjacency matrix, node features, a pre-trained model to optimize these masks.

\begin{figure}
    \centering
    \includegraphics[width=0.5\textwidth]{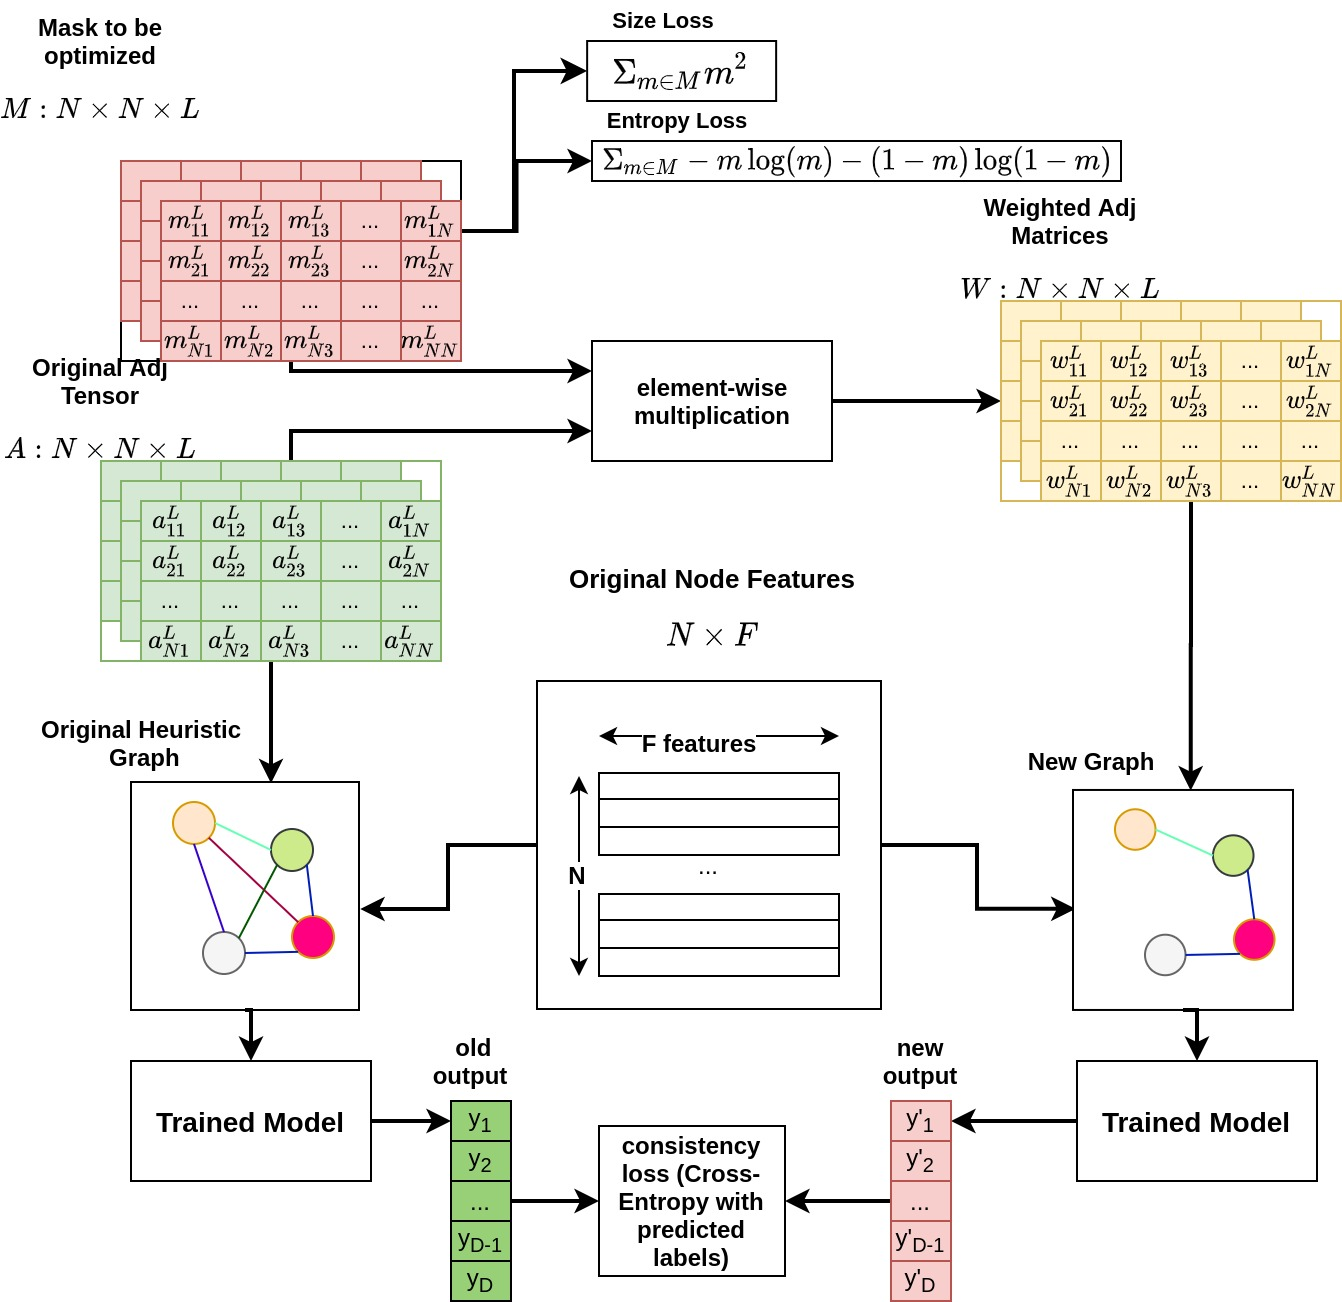}
    \caption{Modified GNN Explainer optimize masks on adjacency tensor: the size loss is used for minimizing size, the entropy loss ensure the mask's tendency to be closer to 0 or 1 while the consistency loss regulate the optimization to keep the prediction unchanged.}
    \label{fig:gnn_explainer_process}
\end{figure}

While the end-goal for explanation is to either debug or to interpret model output, we see that the given subgraphs and feature masks can be used to provide interpretable classification and used as materials to train program synthesis recognition model. 
For the problem of information extraction, we modified original GNN Explainer \cite{Crammer2020} to take input as an adjacency tensor and used 3 type of loss as in Figure \ref{fig:gnn_explainer_process}.

%\subsection{Explore/Compress/Compile}
\textbf{Domain Specific Language (DSL) and Program Synthesis.} The Explore-Compress-Compile ($\text{EC}^2$) is an algorithm to learns Domain Specific Language (DSL) and trains a recognition neural network for program searching\cite{Ellis}. $\text{EC}^2$ takes input as a set of tasks, and efficiently learns solving tasks progressively:
\begin{itemize}
 \item The Exploration phase consist of searching for program solving tasks under guiding of recognition model
 \item Compress refers to finding reused substructures among solved tasks and adding them to the library to reduce the search time for the next searches.
 \item Compile phase refers to training recognition model to guide the enumerative search.
\end{itemize}

\marc{make it concise}
Given a set of tasks, $EC^2$ framework is expected to gradually expand the library and solve the tasks in increased-complexity order.

In order to be able to expand the library, it is required that under the exploration steps a portion of tasks has to be solved.
The works currently focus on typical single-domain tasks such as text-editing, list-processing, etc. 
% We believe the ability to automatically leverages priors knowledge from solved program to learn DSL will be very useful in solving complicated problem of Information Extraction, given that the cost of designing tasks to capture domain-specific knowledge can be alleviated.

Our works aim to solve this gap by having the tasks automatically designed to capture GNN distilled knowledge to learn relevant reusable programs while boosting the performance of Information Extraction, this will be discussed in the next section.

\begin{figure}
    \centering
    \includegraphics[width=0.5\textwidth]{images/MultiPerceptron-GNNArchitecture(2).jpg}
    \caption{Employed Graph Neural Network Architecture, $GConv$ is the graph convolution layer, $Embedding$ is a linear layer per node feature, $Concat$ concatenate node-wise features}
    \label{fig:gnn_architecture}
\end{figure}

\textbf{Architecture: } After all text line features are extracted and the document graph is built, we employed a GNN Architecture of total 5 Graph Convolution (GCN) Layer \cite{Kipf2017, Such2017} in Figure \ref{fig:gnn_architecture}, each are activated by ReLU activation \cite{AlexNet}. Skip connections are also used under the form of concatenation to facilitate gradient flows during training. 
The final layer is an embedding layer to map from per-node aggregated features to available classes.
