# Supplementary material for: VRDSynth: Synthesizing Programs for Multilingual Visually Rich Document Information Extraction
Source: arXiv:2407.06826 source file (2024-07-09)
Supplement: Supplementary file 2 [file supplement_rtree.tex]

\textbf{Graph-based Information Extraction Explanation Via Rules: } We convert GNN Explainer output (adjacency mask and feature masks of nodes) into recognition rules of text lines via the algorithm described in Algorithm \ref{algo:tree_path}. The resulting tree contains keywords as well as children set based on spatial relations is used to be converted to rule in Algorithm \ref{algo:tree_path_to_rule}.

\kai{what are keyword and children? is it key-values?}

\kai{explain algorithm 1 and 2 by words, about how they performs the task. Pseudo code is not the best way to explain idea. For example, how to obtain rules from gnn explainer results. 
Also, algo2 sub-function can be named for easy understanding like text(x), boundingbox(x) then can skip definition mappings. What is the role of lefts, rights, tops, downs?}

\begin{algorithm}
\SetAlgoLined
\KwResult{Relation Tree from main node}
\SetKwInOut{Input}{input}
\Input{
$A \in \{0; 1; 2; 3; 4\} ^ {N \times N}$: Quantized adjacency matrix obtained by combining masks of GNN Explainer. $A_{ij}$ describe having no relation, top, down, left, right \newline
$F \in \{0; 1\} ^ {N(N_w + 4)}$ obtained by thresholding GNN Explainer masked feature, describe whether a feature is important to the prediction. \newline
$C$ - Corpus - list of chosen words from data.
$l\_box$ - List of document boxes with corresponding indices \newline
$i$ - Index of explained node. \newline
}
\Begin {
 $l\_rtree$ $\leftarrow$ $\left[new\ \mathbf{RTree}\ \textbf{for}\ box \in l\_box\right]$\;
 $l\_widx$ $\leftarrow$ GetWordIndices($F[i] == 1$)\;
 $l\_rtree[i].kwrds$ $\leftarrow$ [$C[w\_idx]$ \textbf{for} $w\_idx$ $\in$ $l\_widx$]\;
 $mask\_taken \leftarrow$ $\left[False\ \textbf{for}\ box \in lbox\right]$\;
 $curr\_idxs \leftarrow [i]$\; $mask\_taken[i] \leftarrow True$\;
 \While{$len(curr\_idxs) > 0$}{
  $next\_idxs \leftarrow []$\;
  \For{$j \in curr\_idxs$}{
    \For{$k \in NonZeroIndices(A[j, :])$}{
        \If{\Not{$mask\_taken[k]$}}{
            $next\_idxs.append(k)$\;
            $l\_rtree[j].children[A[j, k] - 1].append(l\_tree[k])$\;
            $mask\_taken[k] \leftarrow True$\;
        }
    }
  }
  $curr\_idxs \leftarrow next\_idxs$\;
 }
 \Return $l\_rtree[i]$\;
 }
 \caption{get\_rtree: Getting Tree Paths from main node}
 \label{algo:tree_path}
\end{algorithm}

After the tree paths is obtained, we proceed converting sample to rule in Algorithm \ref{algo:tree_path_to_rule}.

\begin{algorithm}
\SetAlgoLined
\KwResult{Lambda function to match with a text line}
\SetKwInOut{Input}{input}
\Input{$rtree$ - Relation Tree from the main node}
\Begin{
 $l\_action \leftarrow [0; 1; 2; 3]$
 $l\_act\_func \leftarrow [traverse\_left, traverse\_right, traverse\_top, traverse\_down]$\;
 $rule \leftarrow \lambda\ x:True$\;
 \For{$kw in rtree.kwrds$}{
    $new\_sub\_rule \leftarrow \lambda\ x: contain\_text(get\_text(x))(kw)$\;
    $rule \leftarrow \lambda\ x: and(rule(x)) (new\_sub\_rule(x))$\;
 }
 $rel\_rule \leftarrow \lambda\ x: True$\;
 \For{$action \in l\_action$}
 {
    \For {$child \in rtree.children[action]$}{
        $rel\_rule\ \leftarrow \newline 
        \lambda\ x:and(rel\_rule(x))( \newline
        \quad any(get\_rule(child))(l\_act\_func(x)) \newline
        )$\;
    }
 }
 \Return $rule \leftarrow \lambda\ x: and(rule(x))(rel\_rule(x))$\;
}
\caption{get\_rule: Converting from tree path to rule}
\label{algo:tree_path_to_rule}
\end{algorithm}

In order to overcome this, we employ post-processing rules synthesized from a deep-learning augmented program synthesis, since the rule-synthesizer is trained across different tasks, it is expected to be able to distill learned rules across tasks, giving a boost in performance.
\marc{Better have a grammar}
\marc{At the begining of each task: What is the goal of each task, then, to achieve this goal, we design these tasks}.
\marc{The goal of this rule-learning and synthesis is to achieve...}
\marc{Use examples instead}
\marc{Each time when we refer to smt in Background, mention it in introduction and explain its purpose}
We formulate the problem of information extraction task for program synthesis as follows:
Given a set of $N$ text lines $\langle t_i \rangle_{(N)}$  represented as tuple of $(id, x, y, w, h, text, tops, downs, lefts, rights)$ for the index in list, coordinates, its text content and lists of related ids respectively, we denote this type of tuple $TDocumentBox$. $id$ is of type $TInt$, while $x, y, w, h$ are of type $TReal$, $text$ is of type $TList(TChar)$ (text is a list of characters) and 
Output is a list of boolean $\langle o_i \rangle_{(N)}, o_i \in \{True, False\}$ for each of the desired fields indicating whether each text line belong to the desired class.
In order to do this, we facilitate the set of primitive lambda function as follows:
\begin{itemize}
    \item $traverse\_left$, $traverse\_right$, $traverse\_top$, $traverse\_down$: $(TDocumentBox, TList(TDocumentBox)) \rightarrow TDocumentBox$: This take a document box and a list containing all text lines belong to a document and get the nearest related box, if there does not exist any related box in the direction, the function return $NULL$.
    \item $get\_text: TDocumentBox \rightarrow TList(TChar)$ get the text content of a text line, will return an empty list if the text line is $NULL$.
    \item $get\_x, get\_y, get\_w, get\_h: TDocumentBox \rightarrow TReal$ get the property of the text line, if given $NULL$ these function will return $-1.0$.
    \item $contain\_char: (list(TChar), Tchar)  \rightarrow TBoolean$ checking whether a text content contains a character.
    \item $greater, equal: (TReal, TReal) \rightarrow TBool$ checking whether a real value is greater than or equal another.
    \item $and, or: (TBoolean, TBoolean) \rightarrow TBoolean; not: TBoolean \rightarrow TBoolean$ - logical functions to combine conditions.
    \item $map: (TVar0 \rightarrow TVar1, TList(TVar0)) \rightarrow TList(TVar1)$ mapping from one type of list to another.
\end{itemize}
